# Supplementary material for: Robust Self-Supervised Extrinsic Self-Calibration
Source: arXiv:2308.02153 source file (2023-08-07)
Supplement: Supplementary file 1 [file suppmat_networks.tex]

\begin{table}[t!]%
\small
  \centering
\resizebox{0.84\linewidth}{!}{
\subfloat[][Depth Network \cite{monodepth2}.]{
%%%%%%%%%%%%%%%%%%%%%%%%%%%%%%%%%%%%%%%%%%%%%%%%%%%
\begin{tabular}[b]{l|l|c|c|c}
\toprule
& \textbf{Layer Description} & \textbf{K} & \textbf{S} & \textbf{Out. Dim.} \\ 
\toprule
\multicolumn{5}{c}{\textbf{ResidualBlock (K, S)}} \\ 
\midrule
\#A & Conv2d $\shortrightarrow$ BN $\shortrightarrow$ ReLU & K & 1 &  \\
\#B & Conv2d $\shortrightarrow$ BN $\shortrightarrow$ ReLU & K & S &  \\
\toprule
\multicolumn{5}{c}{\textbf{UpsampleBlock (\#skip)}} \\ 
\midrule
\#C & Conv2d $\shortrightarrow$ BN $\shortrightarrow$ ReLU $\shortrightarrow$ Upsample         & 3 & 1 & \\
\#D & Conv2d ($\#C \oplus \#skip$) $\shortrightarrow$ BN $\shortrightarrow$ ReLU  & 3 & 1 & \\
\toprule
\toprule
\#0 & Input RGB image & - & - & 3$\times$H$\times$W \\ 
\midrule
\multicolumn{5}{c}{\textbf{Encoder}} \\ \hline
\#1  & Conv2d $\shortrightarrow$ BN $\shortrightarrow$ ReLU   & 7 & 1 &  64$\times$H$\times$W \\
\#2  & Max. Pooling                 & 3 & 2 &  64$\times$H/2$\times$W/2 \\
\#3  & ResidualBlock (x2)           & 3 & 2 &  64$\times$H/4$\times$W/4 \\
\#4  & ResidualBlock (x2)           & 3 & 2 & 128$\times$H/8$\times$W/8 \\
\#5  & ResidualBlock (x2)           & 3 & 2 & 256$\times$H/16$\times$W/16 \\
\#6  & ResidualBlock (x2)           & 3 & 2 & 512$\times$H/32$\times$W/32 \\
\midrule
\multicolumn{5}{c}{\textbf{Depth Decoder}} \\ 
\midrule
\#7 & UpsampleBlock (\#5)    & 3 & 1 & 256$\times$H/16$\times$W/16 \\
\#8 & UpsampleBlock (\#4)    & 3 & 1 & 128$\times$H/8$\times$W/8 \\
\#9 & UpsampleBlock (\#3)    & 3 & 1 & 64$\times$H/4$\times$W/4 \\
\#10 & UpsampleBlock (\#2)   & 3 & 1 & 32$\times$H/2$\times$W/2 \\
\#11 & UpsampleBlock (\#1)   & 3 & 1 & 32$\times$H$\times$W \\
\#12 & Conv2d $\shortrightarrow$ Sigmoid  & 3 & 1 & 1$\times$H$\times$W \\
\bottomrule
\end{tabular}
\label{tab:netdepth}
}}
\\
\resizebox{0.84\linewidth}{!}{
\subfloat[][Pose Network \cite{zhou2018unsupervised}.]{
\begin{tabular}[b]{l|c|c|c|c}
\toprule
& \textbf{Layer Description} & \textbf{K} & \textbf{S} & \textbf{Out. Dim.} \\ 
\toprule
\#0 & Input 2 RGB images & - & - & 6$\times$H$\times$W \\ 
\midrule
\#1  & \hspace{2mm} Conv2d $\shortrightarrow$ GN $\shortrightarrow$ ReLU \hspace{2mm} & 3 & 2 & 16$\times$H/2$\times$W/2 \\
\#2  & \hspace{2mm} Conv2d $\shortrightarrow$ GN $\shortrightarrow$ ReLU \hspace{2mm} & 3 & 2 & 32$\times$H/4$\times$W/4 \\
\#3  & \hspace{2mm} Conv2d $\shortrightarrow$ GN $\shortrightarrow$ ReLU \hspace{2mm} & 3 & 2 & 64$\times$H/8$\times$W/8 \\
\#4  & \hspace{2mm} Conv2d $\shortrightarrow$ GN $\shortrightarrow$ ReLU \hspace{2mm} & 3 & 2 & 128$\times$H/16$\times$W/16 \\
\#5  & \hspace{2mm} Conv2d $\shortrightarrow$ GN $\shortrightarrow$ ReLU \hspace{2mm} & 3 & 2 & 256$\times$H/32$\times$W/32 \\
\#6  & \hspace{2mm} Conv2d $\shortrightarrow$ GN $\shortrightarrow$ ReLU \hspace{2mm} & 3 & 2 & 256$\times$H/64$\times$W/64 \\
\#7  & \hspace{2mm} Conv2d $\shortrightarrow$ GN $\shortrightarrow$ ReLU \hspace{2mm} & 3 & 2 & 256$\times$H/128$\times$W/128 \\
\#8  & Conv2d & 1 & 1 & 6$\times$H/128$\times$W/128 \\
\midrule
\#9  & Global Pooling & - & - & 6 \\
\bottomrule
\end{tabular}
\label{tab:netpose}
}}
\\
%%%%%%%%%%%%%%%%%%%%%%%%%%%%%%%%%%%%%%%%%%%%%%%%%%%
\caption{
\textbf{Neural network architectures used in our proposed FSM framework}. The predicted depth maps are $1 \times H \times W$ tensors, and the predicted poses are $6$-dimensional vectors representing translation ($x,y,z$) and Euler rotation angles (pitch, yaw, roll).  \emph{BN} stands for Batch Normalization \cite{ioffe2015batch}, \emph{GN} for Group Normalization \cite{WuH18}, \emph{Upsample} doubles spatial dimensions using bilinear interpolation, and \emph{ReLU} denote Rectified Linear Units. The symbol $\oplus$ indicates feature concatenation. 
}
%%%%%%%%%%%%%%%%%%%%%%%%%%%%%%%%%%%%%%%%%%%%%%%%%%%
\label{tab:networks}
\vspace{-5mm}
\end{table}
